# Supplementary material for: Graph Sampling for Matrix Completion Using Recurrent Gershgorin Disc Shift
Source: arXiv:1906.01087 source file (2019-10-16)
Supplement: Supplementary file 1 [file appendix0.tex]

\subsection{Optimality Relation between (\ref{eq:discAlign}) and (\ref{eq:discAlign2})}
\label{subsec:append1}

We show that if $\delta_{\min}$ is chosen such that at least one optimal solution $(\{s_i^*\}, \{e_i^*\})$ to (\ref{eq:discAlign2}) satisfies $\sum_{i=1}^N e_i^* = \bar{H}$, then there also exists one optimal solution to (\ref{eq:discAlign2}) that is the optimal solution to (\ref{eq:discAlign}). 
First, note that all solutions $(\{s_i\}, \{e_i\})$ with sample size $\sum_{i=1}^N e_i > \bar{H}$ are infeasible solutions to (\ref{eq:discAlign}).
Second, for each solution $(\{s_i\}, \{e_i\})$ with sample size $\sum_{i=1}^N e_i < \bar{H}$ satisfying all constraints in (\ref{eq:discAlign2}) except $c_i - r_i \geq \delta_{\min}, \forall i$, we know its smallest Gershgorin disc left-end $\min_i c_i - r_i < \delta_{\min}$, thus is infeasible in  (\ref{eq:discAlign2}).
This is because by assumption one optimal solution $(\{s_i^*\}, \{e_i^*\})$ to (\ref{eq:discAlign2}) has sample size $\sum_{i=1}^N e_i^* = \bar{H}$, and having another feasible solution $(\{s_i\}, \{e_i\})$ in (\ref{eq:discAlign2}) with sample size $\sum_{i=1}^N e_i < \bar{H}$ would contradict this assumption.
This means that while both $(\{s_i^*\}, \{e_i^*\})$ and $(\{s_i\}, \{e_i\})$ are feasible in (\ref{eq:discAlign}), $(\{s_i^*\}, \{e_i^*\})$ has a larger objective value (thus a better solution).
Thus, there must exist one solution $(\{s_i^*\}, \{e_i^*\})$ to (\ref{eq:discAlign2}) with sample size $\sum_{i=1}^N e_i^* = \bar{H}$ that is also optimal to (\ref{eq:discAlign}). $\Box$

\subsection{Non-decreasing Function $H(\delta_{\min})$}
\label{subsec:append2}

We prove that $H(\delta_{\min})$ is a non-decreasing function with respect to $\delta_{\min}$. 
Specifically, given two optimal solutions $(\{s_i^{(1)}\}, \{e_i^{(1)}\})$ and $(\{s_i^{(2)}\}, \{e_i^{(2)}\})$ corresponding to threshold $\delta^{(1)}$ and $\delta^{(2)}$ where $\delta^{(1)} < \delta^{(2)}$, we show that $H(\delta^{(1)}) \leq H(\delta^{(2)})$.
We prove by contradiction: 
suppose instead that $H(\delta^{(1)}) = \sum_{i=1}^N e_i^{(1)} > H(\delta^{(2)}) =\sum_{i=1}^N e_i^{(2)}$.
First, optimal solution $(\{s_i^{(2)}\}, \{e_i^{(2)}\})$ to (\ref{eq:discAlign2}) given threshold $\delta^{(2)}$ must be feasible and satisfies all constraints. 
This solution $(\{s_i^{(2)}\}, \{e_i^{(2)}\})$ is also feasible given threshold $\delta^{(1)}$, since $c_i - r_i \geq \delta^{(2)}, \forall i$ implies $c_i - r_i \geq \delta^{(2)} > \delta^{(1)}, \forall i$.
However, solution $(\{s_i^{(2)}\}, \{e_i^{(2)}\})$ being feasible when threshold is $\delta^{(1)}$ violates the optimality of $(\{s_i^{(1)}\}, \{e_i^{(1)}\})$, since by assumption $\sum_{i=1}^N e_i^{(1)} > \sum_{i=1}^N e_i^{(2)}$, and  solution $(\{s_i^{(2)}\}, \{e_i^{(2)}\})$ has a strictly smaller objective. This is a contradiction. $\Box$
